# Supplementary material for: A Novel Bayesian Extrapolation Design for Assessing Equivalence in Exposure-Response Curves between Pediatric and Adult Populations
Source: arXiv:2505.17397 ancillary file (2025-05-23)
Supplement: Supplementary file 1 [file supplement.pdf]

Biometrics ,

# Supplementary Material for "A Novel Bayesian Extrapolation Design for Assessing Equivalence in Exposure-Response Curves between Pediatric and Adult Populations "

**Zhongheng Cai**

Department of Biostatistics, St. Jude Children's Research Hospital, Memphis, USA

**and**

**Lian Ma**

Createrna Science and Technology, Gaithersburg, Maryland, USA

**and**

**Jingjing Ye**

Global Statistics and Data Science at BeiGene, Washington DC, USA

**email:* jingjing.ye@beigene.com

**and**

**Haitao Pan**

Department of Biostatistics, St. Jude Children's Research Hospital, Memphis, USA

**email:* Haitao.Pan@stjude.org

This paper has been submitted for consideration for publication in *Biometrics*

**Web Appendix A: Supporting information referenced in Sections 2.2: Workflow**

Web Figure 1 illustrates workflow of generating $\boldsymbol{\beta}_{\text{ped}}$ in Section 2.2.

[Web Figure 1 about here.]

**Web Appendix B: Supporting information referenced in Section 5.2: Sensitivity Analysis**

In the manuscript, we consider the following scenarios to test the stability of our parameter choices:

(1). **Changing Weights for $\boldsymbol{\eta}$:** We altered the weights for $\pi_0(\boldsymbol{\eta})$ and $\pi_1(\boldsymbol{\eta})$ to be (4,2,2,1,1,1,1,1,1,1) and (1,1,1,1,1,1,1,1,2,2,4), respectively. This case represents an increased probability of selecting the elements of $\boldsymbol{\eta}$ with weight 1, thereby expanding the search space for $\boldsymbol{\eta}$.

(2). **Modified Probability Ratios:** We adjusted the ratio of the probability of $x \in [a, b]$ to $x \in [A, B] - [a, b]$ by doubling it, aiming to better reflect real-world conditions, namely, the exposure in pediatric population will concentrate on high level.

(3). **Magnitude of Difference in REPP for $\boldsymbol{\beta}_{\textbf{ped}}$:** We assume that the mean of deviation at each point in $\boldsymbol{x} = (2.5, 3.125, 4.375)$ is 10% or 15% of the corresponding adult E-R log odds ratio. For 10%, we call it a moderate difference, and for 15%, we call it a large difference. We expected that the larger difference would lead to lower type I error and reduced power. These cases reflect different beliefs about the similarity of E-R relationships between the pediatric and adult populations: greater bias corresponds to greater dissimilarity.

Scenario 1 examines the effect of changing weights. In Section 4 of manuscript, we initially chose a configuration where the largest weight was eight times the smallest. Results presented in Supplementary Table 1, compared with Table 1 in the manuscript, show that most candidate selections remain the same, indicating that the choice of weight has minimal

impact on the final parameter selection. Additionally, both tables illustrate a trend. With larger sample sizes, we may find that they share majority of the same candidate designs, which means that the choice of the weight has little effect on the final design. Furthermore, both tables display a trend where larger sample sizes (e.g., $n = 64$) typically exhibit higher power and lower Type I error rates compared to smaller sample sizes (e.g., $n = 40$) for the same $\epsilon_{\text{bayes}}$ and $w$. Scenario 2 focuses on doubling the probability that the exposure falls within the interval of interest, aiming to better mimic practical conditions. Results in Supplementary Table 2 indicate a general decrease in Type I error and power compared to Table 1 in the manuscript. For combinations of, $(n, w, \epsilon_{\text{bayes}})$, the selections remain consistent when $\epsilon_{\text{bayes}} = 0.95$ while is much more different when $\epsilon_{\text{bayes}} = 0.99$, which is likely due to the reduction in power. Scenario 3 evaluates the impact of using the smaller or larger difference REPP. Results of moderate difference and large difference in Supplementary Table 3, compared with Table 1 in the manuscript, show that Type I error and power are relatively small. However, when $\epsilon_{\text{bayes}} = 0.95$, all the three tables have almost identical admissible design tuples when sample size $n \geqslant 45$, which lead to the same final decision.

To summarize all the scenarios, the final candidate selections are consistent for $\epsilon_{\text{bayes}} = 0.95$, which means that we have the same final choice of $(n, w, \epsilon_{\text{bayes}})$. The result shows that our method has a stable choice of $(n, w, \epsilon_{\text{bayes}})$.

[Web Table 1 about here.]

[Web Table 2 about here.]

[Web Table 3 about here.]

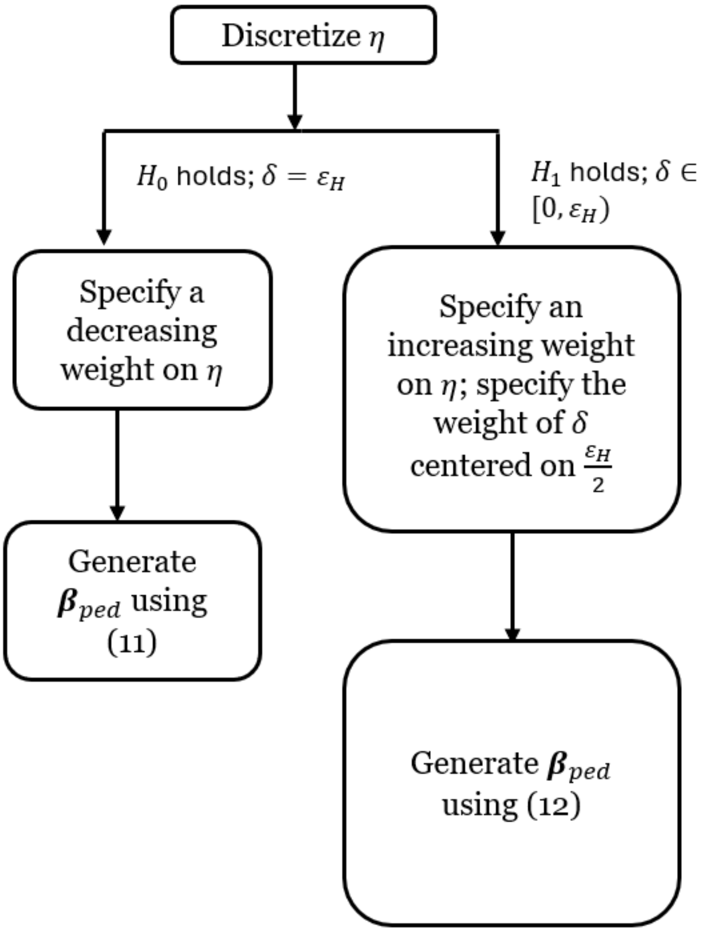


**Figure 1**: Workflow to generate the $\boldsymbol{\beta}_{\text{ped}}$

| sample size | $w$ \ $\epsilon_{\text{bayes}}$ | 0.8 | 0.85 | 0.9 | 0.95 | 0.99 |
|---|---|---|---|---|---|---|
| $n = 40$ | 0.1 | (0.425,0.875) | (0.360,0.840) | (0.275,0.760) | (0.160,0.656) | (0.030,0.385) |
| | 0.2 | (0.630,0.925) | (0.570,0.885) | (0.435,0.860) | (0.255,0.785) | (0.045,0.540) |
| | 0.3 | (0.630,0.950) | (0.565,0.920) | (0.455,0.895) | (0.320,0.790) | (0.095,0.610) |
| | 0.4 | (0.720,0.975) | (0.630,0.960) | (0.535,0.935) | (0.395,0.870) | (0.120,0.615) |
| | 0.5 | (0.715,0.955) | (0.630,0.940) | (0.500,0.920) | (0.325,0.855) | (0.105,0.645) |
| $n = 45$ | 0.1 | (0.465,0.885) | (0.370,0.865) | (0.29,0.820) | (0.190,0.74) | (0.050,0.430) |
| | 0.2 | (0.545,0.935) | (0.440,0.925) | (0.370,0.865) | (0.230,0.76) | (0.100,0.535) |
| | 0.3 | (0.630,0.930) | (0.550,0.900) | (0.440,0.880) | (0.315,0.82) | (0.085,0.560) |
| | 0.4 | (0.690,0.940) | (0.645,0.930) | (0.550,0.895) | (0.350,0.86) | (0.125,0.620) |
| | 0.5 | (0.725,0.970) | (0.655,0.950) | (0.585,0.930) | (0.455,0.860) | (0.175,0.605) |
| $n = 50$ | 0.1 | (0.400,0.920) | (0.350,0.885) | (0.265,0.85) | (0.165,0.720) | (0.040,0.475) |
| | 0.2 | (0.515,0.925) | (0.455,0.910) | (0.345,0.880) | (0.245,0.820) | (0.07,0.535) |
| | 0.3 | (0.615,0.930) | (0.540,0.920) | (0.435,0.880) | (0.295,0.840) | (0.100,0.640) |
| | 0.4 | (0.595,0.945) | (0.530,0.940) | (0.470,0.920) | (0.355,0.835) | (0.13,0.625) |
| | 0.5 | (0.700,0.975) | (0.650,0.965) | (0.520,0.940) | (0.345,0.905) | (0.12,0.690) |
| $n = 55$ | 0.1 | (0.525,0.870) | (0.410,0.835) | (0.340,0.795) | (0.195,0.68) | (0.025,0.475) |
| | 0.2 | (0.525,0.910) | (0.445,0.890) | (0.390,0.855) | (0.295,0.770) | (0.115,0.545) |
| | 0.3 | (0.665,0.965) | (0.595,0.965) | (0.505,0.945) | (0.355,0.860) | (0.170,0.680) |
| | 0.4 | (0.595,0.950) | (0.505,0.935) | (0.435,0.910) | (0.330,0.850) | (0.115,0.615) |
| | 0.5 | (0.66,0.930) | (0.600,0.920) | (0.535,0.900) | (0.410,0.86) | (0.135,0.610) |
| $n = 60$ | 0.1 | (0.460,0.865) | (0.405,0.840) | (0.315,0.79) | (0.215,0.70) | (0.065,0.475) |
| | 0.2 | (0.505,0.920) | (0.435,0.905) | (0.320,0.86) | (0.220,0.750) | (0.065,0.535) |
| | 0.3 | (0.510,0.890) | (0.470,0.880) | (0.385,0.85) | (0.245,0.810) | (0.065,0.630) |
| | 0.4 | (0.700,0.960) | (0.630,0.950) | (0.550,0.93) | (0.355,0.885) | (0.090,0.635) |
| | 0.5 | (0.645,0.950) | (0.580,0.925) | (0.515,0.915) | (0.315,0.835) | (0.110,0.665) |
| $n = 64$ | 0.1 | (0.410,0.875) | (0.360,0.845) | (0.275,0.800) | (0.185,0.75) | (0.070,0.530) |
| | 0.2 | (0.445,0.930) | (0.375,0.925) | (0.310,0.900) | (0.185,0.805) | (0.035,0.590) |
| | 0.3 | (0.535,0.920) | (0.450,0.900) | (0.395,0.870) | (0.280,0.805) | (0.090,0.60) |
| | 0.4 | (0.700,0.960) | (0.635,0.940) | (0.515,0.910) | (0.300,0.85) | (0.105,0.68) |
| | 0.5 | (0.615,0.965) | (0.555,0.960) | (0.465,0.935) | (0.315,0.895) | (0.085,0.70) |

Table 1: Sensitivity analysis: In $\pi_0(\boldsymbol{\eta})$ and $\pi_1(\boldsymbol{\eta})$, the highest probability is four times the lowest probability. First number in the bracket is type I error. Second number is the power. The red numbers are the pairs satisfying the type I and II error constraint. Blue ones are the potential candidates. The results are based on $\epsilon_H = 0.2$.

| sample size | $w$ \ $\epsilon_{\text{bayes}}$ | 0.8 | 0.85 | 0.9 | 0.95 | 0.99 |
|---|---|---|---|---|---|---|
| $n = 40$ | 0.1 | (0.415,0.870) | (0.315,0.825) | (0.210,0.775) | (0.125,0.685) | (0.030,0.350) |
| | 0.2 | (0.590,0.910) | (0.515,0.895) | (0.440,0.860) | (0.285,0.755) | (0.075,0.495) |
| | 0.3 | (0.675,0.915) | (0.600,0.890) | (0.510,0.850) | (0.370,0.755) | (0.135,0.495) |
| | 0.4 | (0.670,0.910) | (0.630,0.890) | (0.495,0.860) | (0.315,0.780) | (0.095,0.510) |
| | 0.5 | (0.725,0.970) | (0.605,0.955) | (0.500,0.905) | (0.355,0.810) | (0.110,0.570) |
| $n = 45$ | 0.1 | (0.420,0.835) | (0.360,0.810) | (0.260,0.750) | (0.155,0.665) | (0.020,0.360) |
| | 0.2 | (0.580,0.880) | (0.515,0.825) | (0.425,0.785) | (0.270,0.685) | (0.085,0.395) |
| | 0.3 | (0.565,0.945) | (0.515,0.930) | (0.425,0.885) | (0.240,0.825) | (0.060,0.570) |
| | 0.4 | (0.690,0.930) | (0.595,0.920) | (0.490,0.915) | (0.365,0.845) | (0.120,0.535) |
| | 0.5 | (0.670,0.945) | (0.630,0.925) | (0.510,0.890) | (0.370,0.830) | (0.125,0.625) |
| $n = 50$ | 0.1 | (0.420,0.870) | (0.345,0.835) | (0.280,0.800) | (0.175,0.700) | (0.055,0.375) |
| | 0.2 | (0.575,0.910) | (0.510,0.890) | (0.400,0.855) | (0.225,0.715) | (0.050,0.460) |
| | 0.3 | (0.600,0.915) | (0.545,0.895) | (0.430,0.850) | (0.280,0.750) | (0.110,0.510) |
| | 0.4 | (0.665,0.950) | (0.615,0.920) | (0.55,0.905) | (0.310,0.845) | (0.080,0.690) |
| | 0.5 | (0.685,0.950) | (0.610,0.935) | (0.50,0.885) | (0.355,0.835) | (0.115,0.600) |
| $n = 55$ | 0.1 | (0.370,0.880) | (0.315,0.855) | (0.220,0.765) | (0.120,0.70) | (0.040,0.470) |
| | 0.2 | (0.525,0.910) | (0.470,0.885) | (0.390,0.830) | (0.250,0.760) | (0.085,0.575) |
| | 0.3 | (0.640,0.920) | (0.550,0.890) | (0.450,0.870) | (0.300,0.805) | (0.115,0.540) |
| | 0.4 | (0.595,0.955) | (0.530,0.950) | (0.425,0.905) | (0.295,0.815) | (0.08,0.610) |
| | 0.5 | (0.585,0.960) | (0.530,0.955) | (0.415,0.920) | (0.290,0.870) | (0.140,0.630) |
| $n = 60$ | 0.1 | (0.395,0.880) | (0.325,0.860) | (0.230,0.810) | (0.145,0.70) | (0.055,0.425) |
| | 0.2 | (0.515,0.930) | (0.465,0.910) | (0.380,0.91) | (0.245,0.795) | (0.060,0.595) |
| | 0.3 | (0.64,0.905) | (0.570,0.875) | (0.420,0.88) | (0.310,0.760) | (0.075,0.625) |
| | 0.4 | (0.595,0.955) | (0.540,0.930) | (0.435,0.93) | (0.305,0.795) | (0.095,0.575) |
| | 0.5 | (0.665,0.920) | (0.565,0.905) | (0.455,0.905) | (0.280,0.830) | (0.125,0.670) |
| $n = 64$ | 0.1 | (0.390,0.895) | (0.325,0.860) | (0.255,0.795) | (0.125,0.710) | (0.025,0.475) |
| | 0.2 | (0.475,0.900) | (0.405,0.875) | (0.300,0.855) | (0.190,0.765) | (0.040,0.605) |
| | 0.3 | (0.555,0.920) | (0.450,0.890) | (0.365,0.860) | (0.255,0.750) | (0.100,0.555) |
| | 0.4 | (0.575,0.940) | (0.505,0.930) | (0.410,0.895) | (0.250,0.835) | (0.085,0.655) |
| | 0.5 | (0.640,0.960) | (0.590,0.945) | (0.470,0.925) | (0.330,0.865) | (0.095,0.645) |

Table 2: Sensitivity analysis: Probability of $x \in [a, b]$ is doubled. First number in the bracket is type I error. Second number is the power. The red numbers are the pairs satisfying the type I and II error constraint. Blue ones are the potential candidates. The results are based on $\epsilon_H = 0.2$.

| sample size | $w$ \ $\epsilon_{\text{bayes}}$ | 0.8 | 0.85 | 0.9 | 0.95 | 0.99 |
|---|---|---|---|---|---|---|
| $n = 40$ | 0.1 | (0.405,0.850) | (0.325,0.830) | (0.245,0.760) | (0.155,0.660) | (0.030,0.385) |
| | 0.2 | (0.620,0.930) | (0.545,0.890) | (0.440,0.860) | (0.285,0.780) | (0.060,0.550) |
| | 0.3 | (0.650,0.945) | (0.585,0.930) | (0.465,0.890) | (0.300,0.795) | (0.110,0.615) |
| | 0.4 | (0.745,0.960) | (0.660,0.930) | (0.570,0.900) | (0.395,0.830) | (0.13,0.585) |
| | 0.5 | (0.730,0.950) | (0.655,0.935) | (0.485,0.925) | (0.315,0.855) | (0.08,0.640) |
| $n = 45$ | 0.1 | (0.445,0.880) | (0.340,0.865) | (0.250,0.815) | (0.155,0.73) | (0.055,0.445) |
| | 0.2 | (0.545,0.930) | (0.45,0.915) | (0.37,0.860) | (0.240,0.77) | (0.10,0.535) |
| | 0.3 | (0.610,0.940) | (0.550,0.925) | (0.445,0.900) | (0.280,0.840) | (0.085,0.580) |
| | 0.4 | (0.690,0.930) | (0.63,0.900) | (0.50,0.875) | (0.340,0.840) | (0.105,0.655) |
| | 0.5 | (0.745,0.970) | (0.680,0.950) | (0.610,0.935) | (0.445,0.85) | (0.175,0.620) |
| $n = 50$ | 0.1 | (0.405,0.915) | (0.330,0.865) | (0.255,0.830) | (0.155,0.725) | (0.050,0.495) |
| | 0.2 | (0.515,0.920) | (0.470,0.900) | (0.360,0.865) | (0.245,0.800) | (0.055,0.545) |
| | 0.3 | (0.630,0.930) | (0.560,0.910) | (0.450,0.900) | (0.300,0.850) | (0.105,0.645) |
| | 0.4 | (0.585,0.945) | (0.520,0.930) | (0.445,0.910) | (0.350,0.845) | (0.125,0.685) |
| | 0.5 | (0.715,0.975) | (0.635,0.960) | (0.520,0.925) | (0.350,0.890) | (0.100,0.675) |
| $n = 55$ | 0.1 | (0.510,0.885) | (0.400,0.855) | (0.325,0.790) | (0.175,0.680) | (0.025,0.455) |
| | 0.2 | (0.550,0.910) | (0.510,0.885) | (0.440,0.860) | (0.265,0.755) | (0.080,0.570) |
| | 0.3 | (0.680,0.970) | (0.625,0.955) | (0.520,0.930) | (0.345,0.85) | (0.155,0.710) |
| | 0.4 | (0.59,0.950) | (0.510,0.935) | (0.435,0.915) | (0.340,0.860) | (0.125,0.620) |
| | 0.5 | (0.660,0.930) | (0.620,0.915) | (0.545,0.900) | (0.370,0.870) | (0.105,0.660) |
| $n = 60$ | 0.1 | (0.455,0.880) | (0.400,0.845) | (0.325,0.81) | (0.205,0.735) | (0.035,0.485) |
| | 0.2 | (0.515,0.915) | (0.455,0.900) | (0.355,0.84) | (0.240,0.76) | (0.075,0.545) |
| | 0.3 | (0.545,0.905) | (0.480,0.895) | (0.405,0.87) | (0.270,0.825) | (0.095,0.620) |
| | 0.4 | (0.695,0.960) | (0.615,0.950) | (0.535,0.940) | (0.360,0.880) | (0.095,0.710) |
| | 0.5 | (0.660,0.955) | (0.590,0.930) | (0.520,0.91) | (0.320,0.855) | (0.110,0.665) |
| $n = 64$ | 0.1 | (0.455,0.885) | (0.375,0.855) | (0.285,0.815) | (0.195,0.755) | (0.055,0.570) |
| | 0.2 | (0.445,0.930) | (0.380,0.930) | (0.330,0.900) | (0.190,0.825) | (0.050,0.605) |
| | 0.3 | (0.525,0.915) | (0.450,0.910) | (0.405,0.860) | (0.30,0.795) | (0.095,0.625) |
| | 0.4 | (0.735,0.945) | (0.650,0.930) | (0.515,0.900) | (0.310,0.900) | (0.080,0.675) |
| | 0.5 | (0.655,0.965) | (0.590,0.960) | (0.500,0.940) | (0.350,0.880) | (0.085,0.685) |

Table 3: Sensitivity analysis: Different prior of $\boldsymbol{\beta}_{\text{ped}}$. First number in the bracket is type I error. Second number is the power. The red numbers are the pairs satisfying the type I and II error constraint. Blue ones are the potential candidates. The results are based on $\epsilon_H = 0.2$.
